# Supplementary material for: Expert-Guided Symmetry Detection in Markov Decision Processes
Source: arXiv:2111.10297 source file (2021-11-19)
Supplement: Supplementary file 1 [file 9-appendix.tex]

\section*{\uppercase{Appendix}}
